# Supplementary material for: Robust Smartphone App Identification Via Encrypted Network Traffic Analysis
Source: arXiv:1704.06099 source file (2017-04-20)
Supplement: Supplementary file 1 [file appendix.tex]

\newpage
\onecolumn

\appendix
\begin{table*}[h!]
\begin{footnotesize}
\begin{center}

\caption{Details of the apps in the AppScanner testing set.} \label{table-app-details}
\begin{tabular}{|>{\hspace{\tabred}}r<{\hspace{\tabred}}|>{\hspace{\tabred}}l<{\hspace{\tabred}}|>{\hspace{\tabred}}l<{\hspace{\tabred}}|l
|>{\hspace{\tabred}}r<{\hspace{\tabred}}|>{\hspace{\tabred}}l<{\hspace{\tabred}}|>{\hspace{\tabred}}l<{\hspace{\tabred}}|
}
\cline{1-3}\cline{5-7} 
%\textbf{\#} &\textbf{App Name} & \textbf{Package Name} & \textbf{Category} & \textbf{Number of Installs} \\
\textbf{\#} &\textbf{Package Name} & \textbf{Number of Installs}& {     }& \textbf{\#} &\textbf{Package Name} & \textbf{Number of Installs}\\
\cline{1-3}\cline{5-7} 
1 & com.amazon.kindle & 100-500 million& & 56 & com.hcg.cok.gp & 10-50 million \\ \cline{1-3}\cline{5-7}
2 & com.dictionary & 10-50 million& & 57 & com.bigkraken.thelastwar & 1-5 million \\ \cline{1-3}\cline{5-7}
3 & com.iconology.comics & 1-5 million& & 58 & com.machinezone.gow & 10-50 million\\ \cline{1-3}\cline{5-7}
4 & com.google.android.gm & 1-5 billion & & 59 & com.myfitnesspal.android & 10-50 million\\ \cline{1-3}\cline{5-7}
5 & com.imo.android.imoim & 50-100 million& & 60 & com.tayu.tau.pedometer & 1-5 million\\ \cline{1-3}\cline{5-7}
6 & kik.android & 50-100 million& & 61 & com.runtastic.android & 10-50 million \\ \cline{1-3}\cline{5-7}
7 & com.facebook.orca & 500 million-1 billion & & 62 & com.northpark.drinkwater & 5-10 million\\ \cline{1-3}\cline{5-7}
8 & com.skype.raider & 500 million-1 billion & & 63 & info.androidz.horoscope & 10-50 million\\ \cline{1-3}\cline{5-7}
9 & com.viber.voip & 100-500 million& & 64 & uk.co.dominos.android & 1-5 million\\ \cline{1-3}\cline{5-7}
10 & com.whatsapp & 1-5 billion& & 65 & com.gumtree.android & 1-5 million\\ \cline{1-3}\cline{5-7}
11 & com.yahoo.mobile.client.android.mail & 100-500 million& & 66 & com.justeat.app.uk & 1-5 million\\ \cline{1-3}\cline{5-7}
12 & com.digidust.elokence.akinator.freemium & 10-50 million& & 67 & com.tinder & 10-50 million\\ \cline{1-3}\cline{5-7}
13 & bbc.iplayer.android & 10-50 million& & 68 & com.mobilemotion.dubsmash & 50-100 million\\ \cline{1-3}\cline{5-7}
14 & air.uk.co.bbc.android.mediaplayer & 10-50 million& & 69 & com.google.android.youtube & 1-5 billion \\ \cline{1-3}\cline{5-7}
15 & com.imdb.mobile & 50-100 million& & 70 & com.mixradio.droid & 1-5 million\\ \cline{1-3}\cline{5-7}
16 & air.ITVMobilePlayer & 5-10 million& & 71 & com.shazam.android & 100-500 million\\ \cline{1-3}\cline{5-7}
17 & com.itv.loveislandapp & 50,000-100,000 & & 72 & com.soundcloud.android & 50-100 million\\ \cline{1-3}\cline{5-7}
18 & com.netflix.mediaclient & 100-500 million & & 73 & com.spotify.music & 50-100 million\\ \cline{1-3}\cline{5-7}
19 & hu.tonuzaba.android & 10-50 million& & 74 & com.cnn.mobile.android.phone & 10-50 million\\ \cline{1-3}\cline{5-7}
20 & com.bskyb.skygo & 1-5 million& & 75 & net.zedge.android & 100-500 million\\ \cline{1-3}\cline{5-7}
21 & tv.twitch.android.app & 1-5 million& & 76 & com.instagram.layout & 10-50 million\\ \cline{1-3}\cline{5-7}
22 & com.miniclip.agar.io & 1-5 million& & 77 & com.zentertain.photoeditor & 50-100 million\\ \cline{1-3}\cline{5-7}
23 & com.yodo1.crossyroad & 10-50 million& & 78 & com.google.android.apps.photos & 1-5 million\\ \cline{1-3}\cline{5-7}
24 & com.imangi.templerun2 & 100-500 million& & 79 & com.dropbox.android & 100-500 million\\ \cline{1-3}\cline{5-7}
25 & com.joycity.warshipbattle & 1-5 million& & 80 & com.google.android.apps.inbox & 5-10 million\\ \cline{1-3}\cline{5-7}
26 & com.prettysimple.criminalcaseandroid & 10-50 million & & 81 & com.microsoft.office.outlook & 10-50 million\\ \cline{1-3}\cline{5-7}
27 & com.rovio.angrybirds & 100-500 million& & 82 & com.surpax.ledflashlight.panel & 100-500 million\\ \cline{1-3}\cline{5-7}
28 & com.nordcurrent.canteenhd & 5-10 million& & 83 & com.amazon.mShop.android.shopping & 10-50 million\\ \cline{1-3}\cline{5-7}
29 & com.umonistudio.tile & 50-100 million& & 84 & com.ebay.mobile & 100-500 million\\ \cline{1-3}\cline{5-7}
30 & com.halfbrick.fruitninjafree & 100-500 million& & 85 & com.groupon & 10-50 million\\ \cline{1-3}\cline{5-7}
31 & com.robtopx.geometryjumplite & 50-100 million& & 86 & com.shpock.android & 5-10 million\\ \cline{1-3}\cline{5-7}
32 & com.boombit.RunningCircles & 1-5 million& & 87 & com.contextlogic.wish & 10-50 million\\ \cline{1-3}\cline{5-7}
33 & com.boombit.Spider & 5-10 million& & 88 & com.badoo.mobile & 50-100 million\\ \cline{1-3}\cline{5-7}
34 & com.kiloo.subwaysurf & 100-500 million& & 89 & com.facebook.katana & 1-5 billion \\ \cline{1-3}\cline{5-7}
35 & com.mobilityware.solitaire & 50-100 million& & 90 & com.google.android.apps.plus & 1-5 billion\\ \cline{1-3}\cline{5-7}
36 & com.leftover.CoinDozer & 50-100 million& & 91 & com.instagram.android & 500 million-1 billion \\ \cline{1-3}\cline{5-7}
37 & com.fivestargames.slots & 5-10 million& & 92 & com.chatous.pointblank & 5-10 million \\ \cline{1-3}\cline{5-7}
38 & com.outplayentertainment.bubbleblaze & 5-10 million & & 93 & com.meetup & 1-5 million\\ \cline{1-3}\cline{5-7}
39 & com.king.candycrushsaga & 100-500 million& & 94 & com.pinterest & 50-100 million\\ \cline{1-3}\cline{5-7}
40 & com.king.candycrushsodasaga & 100-500 million& & 95 & com.snapchat.android & 100-500 million\\ \cline{1-3}\cline{5-7}
41 & com.playfirst.cookingdashx & 1-5 million& & 96 & com.twitter.android & 100-500 million\\ \cline{1-3}\cline{5-7}
42 & com.gameloft.android.ANMP.GloftDMHM & 100-500 million& & 97 & com.qihoo.security & 100-500 million\\ \cline{1-3}\cline{5-7}
43 & air.com.puffballsunited.escapingtheprison & 5-10 million& & 98 & com.adobe.air & 100-500 million\\ \cline{1-3}\cline{5-7}
44 & com.king.farmheroessaga & 100-500 million& & 99 & com.cleanmaster.mguard & 100-500 million\\ \cline{1-3}\cline{5-7}
45 & com.outfit7.mytalkingtomfree & 100-500 million& & 100 & com.lazyswipe & 50-100 million\\ \cline{1-3}\cline{5-7}
46 & com.jellybtn.cashkingmobile & 10-50 million& & 101 & com.avast.android.mobilesecurity & 100-500 million\\ \cline{1-3}\cline{5-7}
47 & me.pou.app & 100-500 million& & 102 & uk.co.nationalrail.google & 1-5 million\\ \cline{1-3}\cline{5-7}
48 & com.king.alphabettysaga & 10-50 million& & 103 & com.thetrainline & 1-5 million\\ \cline{1-3}\cline{5-7}
49 & com.ciegames.RacingRivals & 10-50 million& & 104 & com.airbnb.android & 5-10 million\\ \cline{1-3}\cline{5-7}
50 & com.igg.android.finalfable & 1-5 million& & 105 & com.booking & 10-50 million\\ \cline{1-3}\cline{5-7}
51 & com.fungames.flightpilot & 1-5 million& & 106 & com.joelapenna.foursquared & 10-50 million\\ \cline{1-3}\cline{5-7}
52 & com.miniclip.eightballpool & 50-100 million& & 107 & com.google.earth & 100-500 million\\ \cline{1-3}\cline{5-7}
53 & com.BitofGame.MiniGolfRetro & 1-5 million& & 108 & com.google.android.apps.maps & 1-5 billion \\ \cline{1-3}\cline{5-7}
54 & com.supercell.boombeach & 10-50 million& & 109 & com.tripadvisor.tripadvisor & 100-500 million\\ \cline{1-3}\cline{5-7}
55 & com.supercell.clashofclans & 100-500 million& & 110 & bbc.mobile.weather & 5-10 million\\ \cline{1-3}\cline{5-7}
\end{tabular}
\end{center}
\end{footnotesize}
\end{table*}
